# Supplementary material for: AnthroNet: Conditional Generation of Humans via Anthropometrics
Source: arXiv:2309.03812 source file (2023-09-07)
Supplement: Supplementary file 1 [file supp_mat_main.tex]

% % \section{Appendix}
% \documentclass[10pt,twocolumn,letterpaper]{article}

% %%%%%%%%%%%%%%%%%%%%%%%%%%%%%%%%%%%%%%%%%%%%%%%%%%%%%%%%%%%%%%%%%%%%%%%%%%%%%%%
% %%%%%%%%%%%%%%% PAPER TYPE  - PLEASE UPDATE FOR FINAL VERSION %%%%%%%%%%%%%%%%%
% %%%%%%%%%%%%%%%%%%%%%%%%%%%%%%%%%%%%%%%%%%%%%%%%%%%%%%%%%%%%%%%%%%%%%%%%%%%%%%%
% % \usepackage[review]{cvpr}      % To produce the REVIEW version
% % \usepackage{cvpr}              % To produce the CAMERA-READY version
% \usepackage[pagenumbers]{cvpr} % To force page numbers, e.g. for an arXiv version


% %%%%%%%%%%%%%%%%%%%%%%%%%%%%%%%%%%%%%%%%%%%%%%%%%%%%%%%%%%%%%%%%%%%%%%%%%%%%%%%
% %%%%%%%%%%%%%%%%%%%%%%%%%%%%%%  STANDARD PACKAGES %%%%%%%%%%%%%%%%%%%%%%%%%%%%%
% %%%%%%%%%%%%%%%%%%%%%%%%%%%%%%%%%%%%%%%%%%%%%%%%%%%%%%%%%%%%%%%%%%%%%%%%%%%%%%%
% % Include other packages here, before hyperref.
% \usepackage{graphicx}
% \usepackage{amsmath}
% \usepackage{amssymb}
% \usepackage{booktabs}
% \usepackage{csvsimple}
% \usepackage[shortlabels]{enumitem}
% % \usepackage[numbers,sort,compress]{natbib} % for other bib styles


% % It is strongly recommended to use hyperref, especially for the review version.
% % hyperref with option pagebackref eases the reviewers' job.
% % Please disable hyperref *only* if you encounter grave issues, e.g. with the
% % file validation for the camera-ready version.
% %
% % If you comment hyperref and then uncomment it, you should deletehttps://www.overleaf.com/project/6310e6316c5fb422272532ef
% % ReviewTempalte.aux before re-running LaTeX.
% % (Or just hit 'q' on the first LaTeX run, let it finish, and you
% %  should be clear).
% \usepackage[pagebackref,breaklinks,colorlinks]{hyperref}


% % Support for easy cross-referencing
% \usepackage[capitalize]{cleveref}
% \crefname{section}{Sec.}{Secs.}
% \Crefname{section}{Section}{Sections}
% \Crefname{table}{Table}{Tables}
% \crefname{table}{Tab.}{Tabs.}


% %%%%%%%%%%%%%%%%%%%%%%%%%%%%%%%%%%%%%%%%%%%%%%%%%%%%%%%%%%%%%%%%%%%%%%%%%%%%%%%
% %%%%%%%%%%%%%%%%%%%%%%%%%%%%%%%% USER PACKAGES %%%%%%%%%%%%%%%%%%%%%%%%%%%%%%%%
% %%%%%%%%%%%%%%%%%%%%%%%%%%%%%%%%%%%%%%%%%%%%%%%%%%%%%%%%%%%%%%%%%%%%%%%%%%%%%%%
% % \usepackage{subfig} % outdated, use subcaption instead
% % \usepackage{rotating}
% % \usepackage{subcaption} %to have subfigures available
% % \usepackage{adjustbox}
% % \usepackage{float}
% \usepackage{multirow}
% % \usepackage[compact]{titlesec}
% % \usepackage[inline]{enumitem}
% % \usepackage{enumerate}
% % % \bibliographystyle{abbrvnat}
% % % \usepackage{algorithm}
% % % \usepackage{algpseudocode}
% \usepackage{xcolor}         % colors
% \usepackage{dsfont}
% \usepackage{mathrsfs}
% \usepackage[group-separator={,}]{siunitx}

% %%%%%%%%%%%%%%%%%%%%%%%%%%%%%%%%%%%%%%%%%%%%%%%%%%%%%%%%%%%%%%%%%%%%%%%%%%%%%%%
% %%%%%%%%%%%%%%%%%%%%%%%%% TAG YOUR CO-AUTHORS LIKE SO %%%%%%%%%%%%%%%%%%%%%%%%%
% %%%%%%%%%%%%%%%%%%%%%%%%%%%%%%%%%%%%%%%%%%%%%%%%%%%%%%%%%%%%%%%%%%%%%%%%%%%%%%%
% \newcommand{\todo}[1]{{\color{red}{}#1}}
% \newcommand{\sujoy}[1]{{\color{magenta}{\bf Sujoy: }#1}}
% \newcommand{\francesco}[1]{{\color{violet}{\bf Francesco: }#1}}
% \newcommand{\salehe}[1]{{\color{cyan}{\bf Salehe: }#1}}
% \newcommand{\shrinath}[1]{{\color{teal}{\bf Shrinath: }#1}}
% \newcommand{\soroosh}[1]{{\color{orange}{\bf Soroosh: }#1}}
% \newcommand{\jonathan}[1]{{\color{pink}{\bf Jonathan: }#1}}
% \newcommand{\jay}[1]{{\color{purple}{\bf Jay: }#1}}
% \newcommand{\peifeng}[1]{{\color{brown}{\bf Peifeng: }#1}}
% \newcommand{\david}[1]{{\color{olive}{\bf David: }#1}}
% \newcommand{\charles}[1]{{\color{green}{\bf Charles: }#1}}
% \newcommand{\mesh}{$\mathcal{X}^A_b$}
% %%%%%%%%%%%%%%%%%%%%%%%%%%%%%%%%%%%%%%%%%%%%%%%%%%%%%%%%%%%%%%%%%%%%%%%%%%%%%%%
% %%%%%%%%%%%%%%%%%%%%%%%%%%%%%%%% PAPER ID  - 6070 %%%%%%%%%%%%%%%%%%%%%%%%%%%%%
% %%%%%%%%%%%%%%%%%%%%%%%%%%%%%%%%%%%%%%%%%%%%%%%%%%%%%%%%%%%%%%%%%%%%%%%%%%%%%%%
% % \def\cvprPaperID{6070} % Salehe's submission
% \def\cvprPaperID{11852} % Francesco's submission - possibly go with this if Salehe is traveling and can't make the supplementary material submission by Nov 18
% \def\confName{CVPR}
% \def\confYear{2023}
% \def\proposed{AnthroNet }

% \begin{document}

% %%%%%%%%%%%%%%%%%%%%%%%%%%%%%%%%%%%%%%%%%%%%%%%%%%%%%%%%%%%%%%%%%%%%%%%%%%%%%%%
% %%%%%%%%%%%%%%%%%%%%%%%%%%%%%%%%%% TITLE %%%%%%%%%%%%%%%%%%%%%%%%%%%%%%%%%%%%%%
% %%%%%%%%%%%%%%%%%%%%%%%%%%%%%%%%%%%%%%%%%%%%%%%%%%%%%%%%%%%%%%%%%%%%%%%%%%%%%%%
% % \title{One Model to Represent Them All, and in the Hidden Space Bind Them}
% \title{Appendix - AnthroNet: Conditional Generation of Humans via Anthropometrics}

% %%%%%%%%%%%%%%%%%%%%%%%%%%%%%%%%%%%%%%%%%%%%%%%%%%%%%%%%%%%%%%%%%%%%%%%%%%%%%%%
% %%%%%%%%%%%%%%%%%%%%%%%%%%% AUTHOR LIST - USE THIS %%%%%%%%%%%%%%%%%%%%%%%%%%%%
% %%%%%%%%%%%%%%%%%%%%%%%%%%%%%%%%%%%%%%%%%%%%%%%%%%%%%%%%%%%%%%%%%%%%%%%%%%%%%%%
% \author{Francesco Picetti$^*$
% \quad
% Shrinath Deshpande$^*$
% \quad
% Jonathan Leban$^*$
% \quad
% Soroosh Shahtalebi$^\dagger$
% \quad
% Jay Patel$^\dagger$
% \\
% Peifeng Jing
% \quad
% Chunpu Wang
% \quad
% Charles Metze III
% \quad
% Sujoy Ganguly$^\S$
% \quad
% Salehe Erfanian Ebadi$^\S$
% \vspace{0.2cm}
% \\
% \vspace{0.1cm}
% \textbf{Unity Technologies}\\
% {
% \tt\small
% \{francesco.picetti,
% shrinath.deshpande, 
% jonathan.leban, 
% soroosh.shahtalebi, 
% jay.patel, 
% \\
% \tt\small 
% peifeng.jing, 
% davidwang, 
% charles.metze, 
% sujoy.ganguly, 
% salehe.erfanianebadi\}@unity3d.com
% }
% }

% %%%%%%%%%%%%%%%%%%%%%%%%%%%%%%%%%%%%%%%%%%%%%%%%%%%%%%%%%%%%%%%%%%%%%%%%%%%%%%%
% %%%%%%%%%%% CVPR AUTHOR LIST - DO NOT USE - THIS FORMAT WASTES SPACE %%%%%%%%%%
% %%%%%%%%%%%%%%%%%%%%%%%%%%%%%%%%%%%%%%%%%%%%%%%%%%%%%%%%%%%%%%%%%%%%%%%%%%%%%%%
% % \author{Francesco Picetti$^*$
% % % Unity Technologies\\
% % % {\tt\small francesco.picetti@unity3d.com}
% % \and
% % Shrinath Deshpande$^*$
% % % Unity Technologies\\
% % % {\tt\small shrinath.deshpande@unity3d.com}
% % \and
% % Jonathan Leban$^*$
% % % Unity Technologies\\
% % % {\tt\small jonathan.leban@unity3d.com}
% % \and
% % Soroosh Shahtalebi$^\dagger$
% % % Unity Technologies\\
% % % {\tt\small soroosh.shahtalebi@unity3d.com}
% % \and
% % Jay Patel$^\dagger$
% % % Unity Technologies\\
% % % {\tt\small jay.patel@unity3d.com}
% % \and
% % Peifeng Jing
% % % Unity Technologies\\
% % % {\tt\small peifeng.jing@unity3d.com}
% % \and
% % Chunpu Wang
% % % Unity Technologies\\
% % % {\tt\small davidwang@unity3d.com}
% % \and
% % Charles Metze III
% % % Unity Technologies\\
% % % {\tt\small charles.metze@unity3d.com}
% % \and
% % Sujoy Ganguly$^\S$
% % % Unity Technologies\\
% % % {\tt\small sujoy.ganguly@unity3d.com}
% % \and
% % Salehe Erfanian Ebadi$^\S$
% % % Unity Technologies\\
% % % {\tt\small salehe.erfanianebadi@unity3d.com}
% % % \\
% % }

% \maketitle

% \appendix

% \section{Design Parameters}\label{supp:design_parameters}
% This section provides a description of all the deep neural networks and the details of the anthropometric measurements introduced in this work.
% \input{09_01_mesh_gen_arch}


% \input{09_02_anthro_measures_details}

% \input{09_03_anthro_regressor}

% \input{09_04_mesh_skinner_rigger_arch}


% \input{09_05_registration_pipeline}

% \section{Extended Experiments and Results}\label{supp:extended_experiments}

% \input{09_06_extended_results}

% \input{09_07_B2A}

% {\small
% \bibliographystyle{ieee_fullname} % orig
% % \bibliographystyle{abbrvnat}
% % \bibliographystyle{abbrv}
% \bibliography{egbib}
% }


% \end{document}
